# Supplementary material for: Geometry-Aware Feature Matching for Large-Scale Structure from Motion
Source: arXiv:2409.02310 source file (2025-05-12)
Supplement: Supplementary file 1 [file X_suppl.tex]

\section{More Experiments in Feature Matching}

In this section, we demonstrate the effectiveness of our proposed geometry optimization module in improving the performance of the detector-free feature matcher without any geometry information from the detector-based method. The fundamental matrix is initialized by the top half of confident matches.  

\begin{figure}[!ht]
  \centering
  \includegraphics[width=0.9\linewidth]{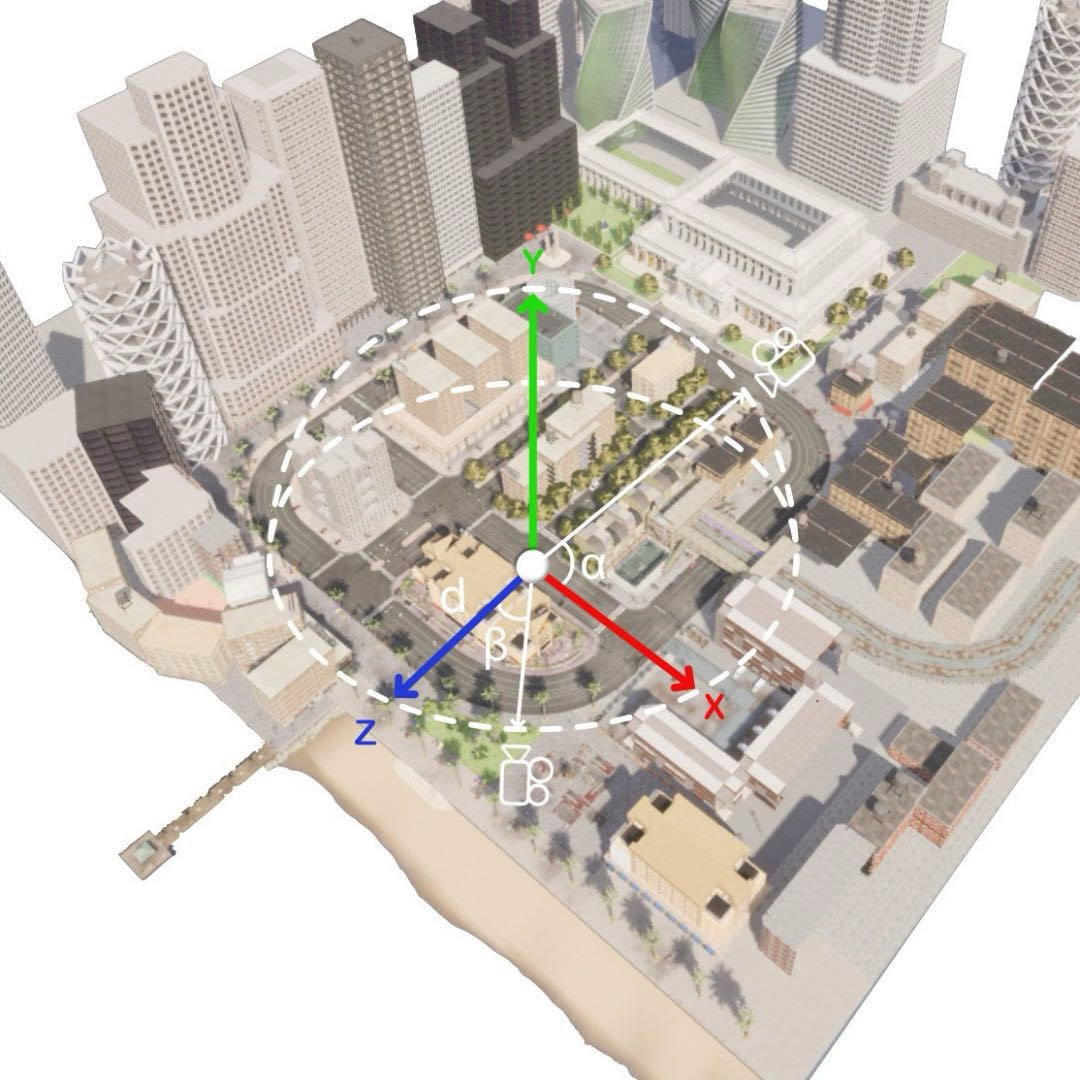}
   \caption{We propose continuous changes along three variable scale/distance $d$ - the radius of the circle, $\alpha$ - the angle between the camera axis and x-axis, $\beta$ - the angle between the projection of the camera axis on xz plane and z-axis. }
   \label{fig:map}
\end{figure}

\subsection{Matching Precision}

\paragraph{Dataset} 

\begin{figure*}[!ht]
  \centering
  \includegraphics[width=1\linewidth]{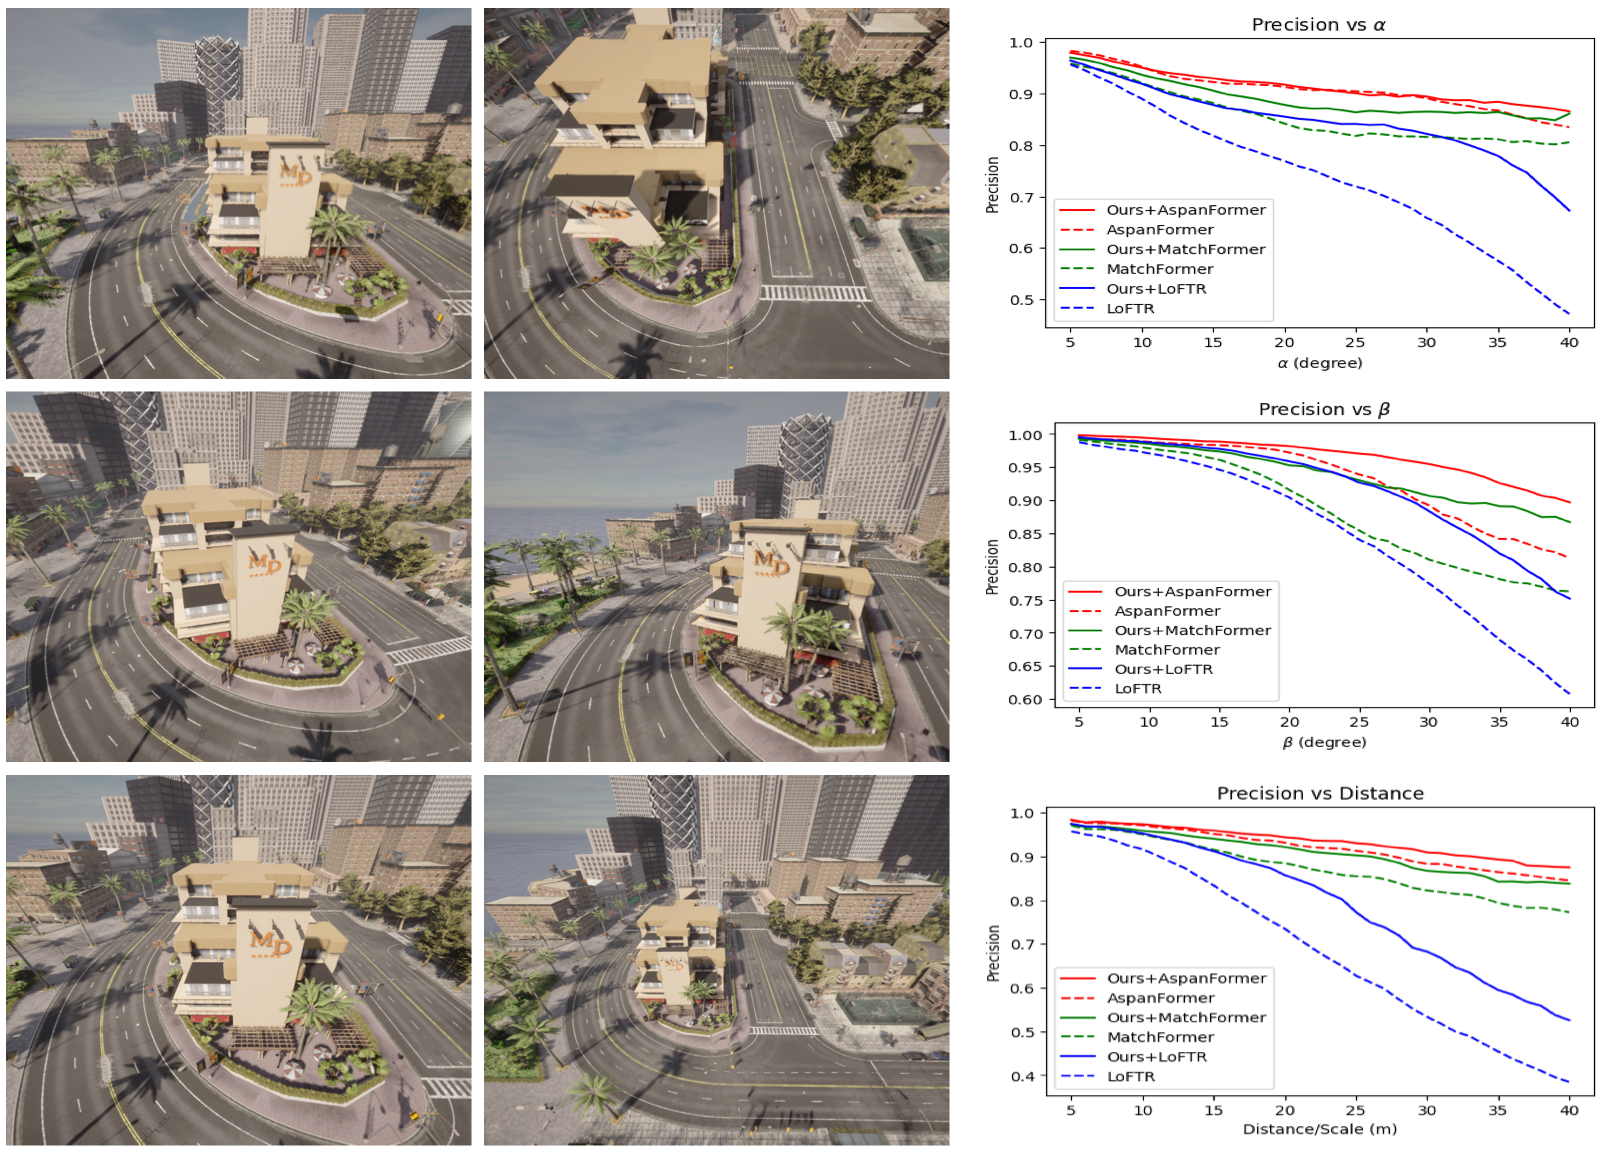}
   \caption{\textbf{Results on our Dataset.} The above illustrates our dataset and the precision evaluation of view changes.  In the first row, $\alpha$ difference ranges from 5$\degree$ to 40$\degree$; in the second row, $\beta$ difference ranges from 5$\degree$ to 40$\degree$; in the third row, distance/scale difference ranges from 5m to 40m. All examples show the largest differences 40$\degree$ for $\alpha$, 40$\degree$ for $\beta$, and 40m for distance. As view differences increase, there is a notable decline in the performance of all methods tested. Notably, our proposed method exhibits superior performance, and the margins of this advantage further escalate with augmented view differences.}
   \label{fig:resultOurData}
\end{figure*}

To understand the performance variations in the context of viewpoint changes, and our proposed optimization module's performance with different detector-free backbones. We generate a synthetic dataset with depth maps and camera poses using CARLA~\cite{Dosovitskiy17}. As illustrated in Figure~\ref{fig:map}, given an image pair $I^A$ and $I^B$, we use the minimum value of a given variable for image $I^A$, 10 for distance, 0 for $\alpha$ and $\beta$. Then we maintain a consistent incremental unit of 1 for such variable for image $I^B$ starting from 5 units of difference, while the other two variables remain the same for both images. We sample 25 image pairs per increment, culminating in a total of 900 image pairs per sequence. Then all images are resized with their longer dimensions adjusted to 832 for the testing. 

\paragraph{Metrics and Comparing Methods}
The average matching precision of 25 image pairs is reported for each step, with correct matches defined based on a symmetric epipolar error threshold of less than $1e^{-4}$. Our methods are compared against three detector-free counterparts, namely LoFTR~\cite{sun2021loftr}, ASpanFormer~\cite{chen2022aspanformer}, and MatchFormer~\cite{wang2022matchformer}. All models are trained on MegaDepth~\cite{li2018megadepth}.

%%%%%%%%%%%%%%%%%%%%%%%%%%%%%%%%%%%%%%%%%%%%%%%%%%%%%%%

\paragraph{Results on Our Dataset.}
For all methods, we observed that the performance drops as the view differences between two images increase, as shown in Figure~\ref{fig:resultOurData}. Our methods consistently outperform the baseline methods, demonstrating a more gradual decline in precision as geometric disparities become more pronounced. While ASpanFormer~\cite{chen2022aspanformer} and MatchFormer~\cite{wang2022matchformer} show robustness against scale variations and changes in the \(\alpha\) angle, they are noticeably impacted by larger \(\beta\) angle differences. This is particularly apparent when the camera that captures image \(I^B\) moves horizontally away from the camera of image \(I^A\), resulting in more significant changes in appearance features compared to the other two scenarios. In contrast, LoFTR~\cite{sun2021loftr}, despite performing adequately under conditions with minimal geometric variation, demonstrates a marked decrease in its ability to find accurate matches as view differences grow.

The integration of our module into these methods has led to substantial improvements in precision. This is indicative of the module's ability to enhance matching accuracy, especially in scenarios where view differences are significant. The result suggests that our approach, by introducing direct geometry constraints early in the matching stage, can mitigate the impact of increasing view geometry challenges.
\setlength\tabcolsep{4.0pt}
\begin{table}[!ht]
    \centering
    \resizebox{0.45\textwidth}{!}{%
    \begin{tabular}{l>{\centering\arraybackslash}m{1.2cm}>{\centering\arraybackslash}m{1.2cm}>{\centering\arraybackslash}m{1.2cm}}
    \toprule
    \multirow{2}{*}{\textbf{Method}}  & \multicolumn{3}{c}{\textbf{AUC} \uparrow} \\
    \cmidrule(lr){2-4}
    & @$3 px$ & @$5 px$ & @$10 px$ \\
    \midrule
    \textit{SuperGlue}~\cite{sarlin20superglue} & 53.9 & 68.3 & 81.7 \\
    \textit{LoFTR}~\cite{sun2021loftr} & 65.9 & 75.6 & 84.6 \\
    \textit{TopicFM}~\cite{giang2023topicfm} & 67.3 & 77.0 & 85.7 \\
    \textit{3DG-STFM}~\cite{mao20223dgstfm} & 64.7 & 73.1 & 81.0 \\
    \textit{ASpanFormer}~\cite{chen2022aspanformer}  & 66.1 & 75.9 & 84.8 \\
    \textit{PDC-Net+}~\cite{truong2021pdcnet} & 66.7 & 76.8 & 85.8 \\
    \textit{Ours-ASpan} & \underline{67.4} & \underline{77.6} & \underline{86.8} \\
    \textit{DKM}~\cite{edstedt2023dkm} & \textbf{71.3} & \textbf{80.6} & \textbf{88.5} \\
    \bottomrule
    \end{tabular}
    }
    \caption{Homography estimation on HPatches, measured in AUC (higher is better).}
    \label{tab:homography}
\end{table}

\begin{figure*}[!ht]
  \centering
  \includegraphics[width=1.0\linewidth]{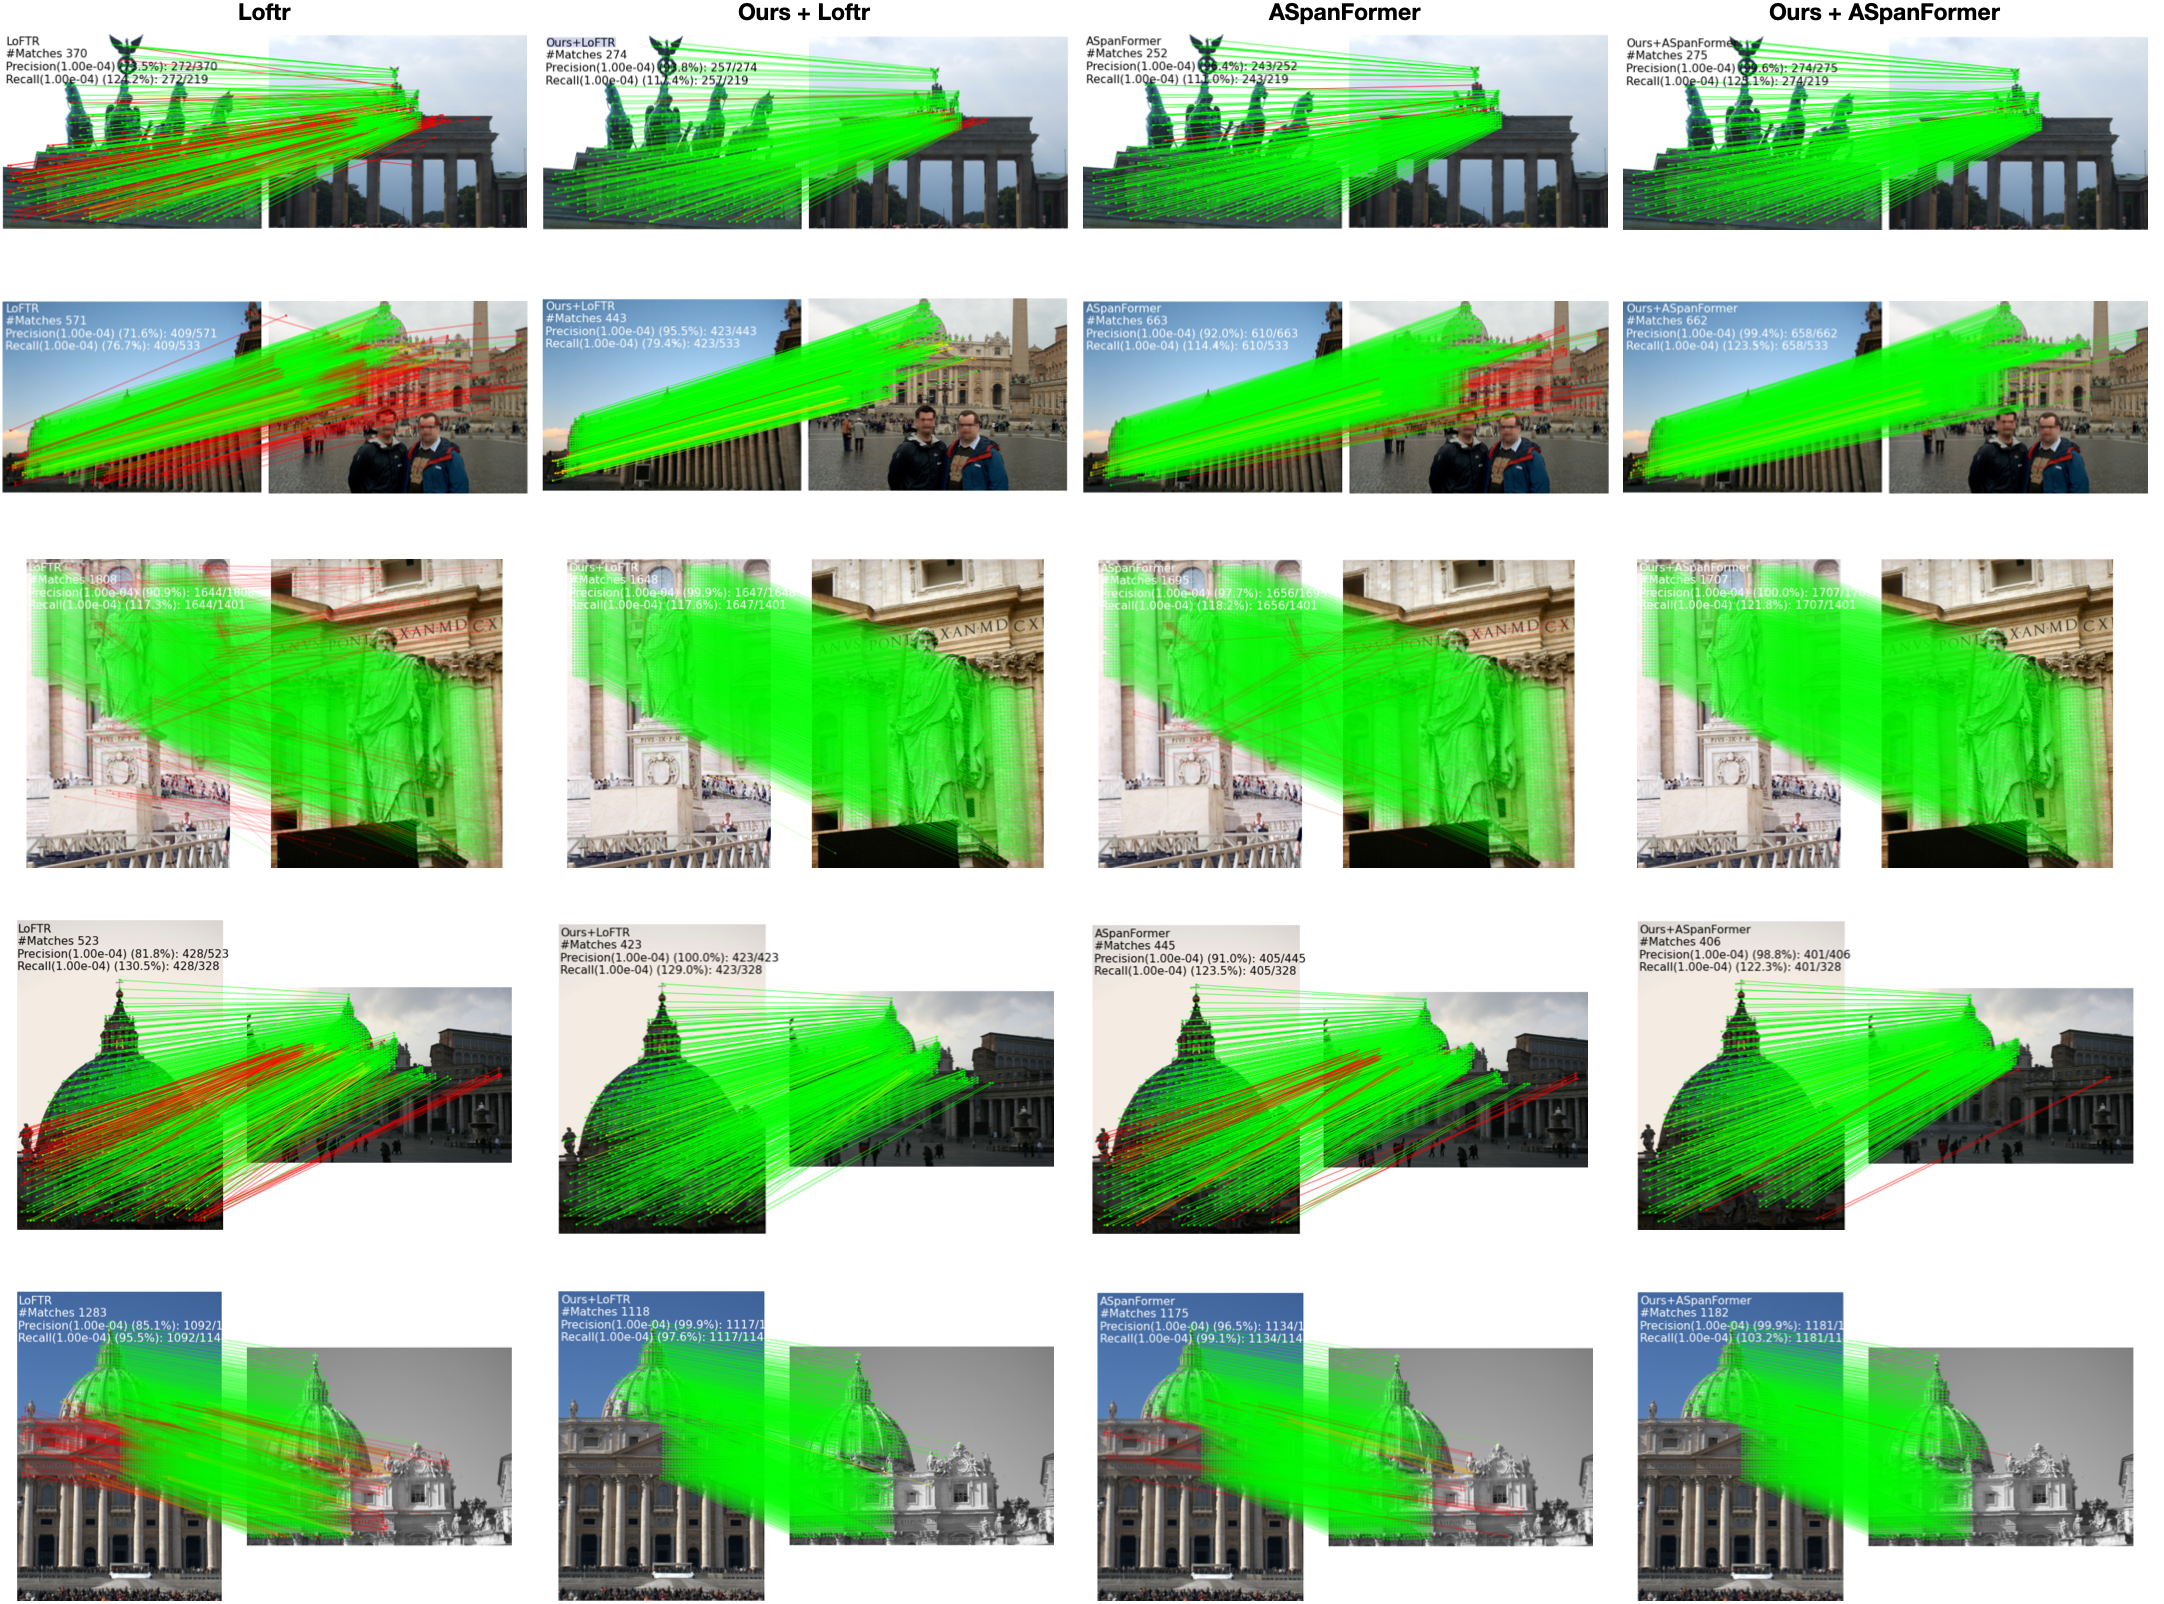}

   \caption{\textbf{Qualitative Results on MegaDepth}. Qualitative Comparison on MegaDepth~\cite{li2018megadepth}. The first column is LoFTR~\cite{sun2021loftr}, the second column is Ours+LoFTR, the third is ASpanFormer and the Forth is Ours+AspanFormer~\cite{chen2022aspanformer}. The green line indicates correct matches in which the symmetric epipolar error is less than $1e^{-4}$, and the red line indicates wrong matches. By introducing the geometry constraints, one can see that the accuracy of matches is improved noticeably.}
   \label{Visualization}
\end{figure*}

\begin{figure*}[!ht]
  \centering
      \includegraphics[width=1\linewidth]{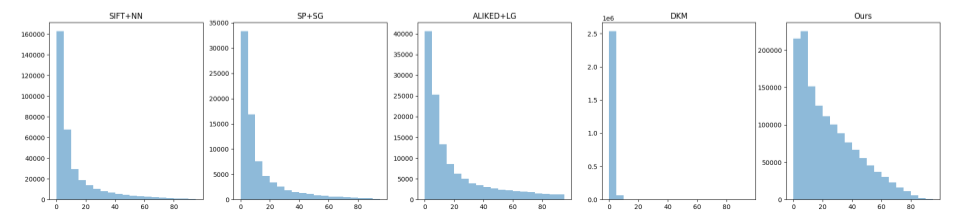}
       \caption{The distribution of track length using different feature matchers on IMC 2021 phototourism dataset ~\cite{Jin2020}}
   \label{fig:track_dist}
\end{figure*}

\subsection{Homography Estimation}

\label{sub:homography}
\paragraph{Datasets} Following~\cite{sun2021loftr,sarlin20superglue,wang2022matchformer}, we evaluate our feature matching method in widely adopted HPatches dataset~\cite{hpatches_2017_cvpr} for homography estimation. Hpatches contain a total of 108 sequences with significant illumination changes and large viewpoint changes. We follow the evaluation protocol of LoFTR~\cite{sun2021loftr}, resizing the shorter size of the image to 480. AUCs at 3 different thresholds are reported.

\paragraph{Results} In Table~\ref{tab:homography}, we can see that our proposed module can improve the performance of our baseline ASpanFormer~\cite{chen2022aspanformer} on HPatches in homography estimation under all error thresholds and only worse than the dense feature matching method DKM~\cite{edstedt2023dkm} which is optimized for two view pose estimation.

\setlength\tabcolsep{4.0pt}
\begin{table}
    \centering
        \begin{tabular}{l>{\centering\arraybackslash}m{1cm}>{\centering\arraybackslash}m{1cm}>{\centering\arraybackslash}m{1cm}}
        \Xhline{1pt}
        \noalign{\smallskip}
        \multirow{2}{*}{\textbf{Method}}  & \multicolumn{3}{c}{\textbf{Pose Estimation AUC} $\uparrow$}\\
        \noalign{\smallskip}
        \cline{2-4}
        \noalign{\smallskip}
        & @$3\degree$ & @$5\degree$ & @$10\degree$ \\
        \noalign{\smallskip}
        \Xhline{1pt}
        \noalign{\smallskip}
        \textit{LoFTR}~\cite{sun2021loftr} & 52.0 & 68.4 & 80.5 \\
        \textit{Ours-LoFTR} & 52.9 & 68.8 & 80.5\\
        \textit{MatchFormer}~\cite{wang2022matchformer} & 51.2 & 68.5 & 81.2\\
        \textit{Ours-MatchFormer} & 52.8 & 69.3 & 81.3 \\
        \textit{ASpanFormer}~\cite{chen2022aspanformer} & 53.0 & 69.8 & 81.8\\
        \textit{Ours-Aspan} & \textbf{55.1} & \textbf{70.9} & \textbf{82.4}\\
        \Xhline{1pt}
    \end{tabular}
    \caption{\textbf{Evaluation on MegaDepth ~\cite{li2018megadepth}} The best performance is highlighted by bold text. The results show that our proposed method can significantly improve the feature matching performance of Detector-free Methods~\cite{sun2021loftr, chen2022aspanformer, wang2022matchformer}}
    \label{megadepth}
\end{table}

\subsection{Relative Pose Estimation}

\paragraph{Dataset} Following ~\cite{sun2021loftr, sarlin20superglue}, we use MegaDepth~\cite{li2018megadepth} for outdoor pose estimation. MegaDepth~\cite{li2018megadepth} is a large outdoor dataset containing over 1 million internet images from 196 different outdoor scenes. The camera pose is reconstructed by COLMAP~\cite{schoenberger2016sfm, schoenberger2016mvs}, and the depth maps are calculated from the multi-view stereo. We follow SuperGlue ~\cite{sarlin20superglue} to obtain the ground truth matches from the depth map and camera pose. We use the same test split as~\cite{sun2021loftr,chen2022aspanformer,wang2022matchformer}. Images are resized such that their longer dimension is equal to 840/832 for training and 832 for testing on all methods. (ASpanFormer~\cite{chen2022aspanformer} use 832 due to their need for an image resolution divisible by 16).

\paragraph{Metrics and Comparing Methods}
We follow SuperGlue~\cite{sarlin20superglue} to report the AUC of recovered pose under threshold (5\degree, 10\degree, and 20\degree). The camera poses are recovered from solving RANSAC with predicted matches. We compared our method to several state-of-the-art methods SuperPoint+SuperGlue~\cite{sarlin20superglue}, LoFTR~\cite{sun2021loftr}, MatchFormer~\cite{wang2022matchformer}, AspanFormer~\cite{chen2022aspanformer}.

\paragraph{Results on MegaDepth} As depicted in Table~\ref{megadepth}, our proposed method outperforms baseline methods. This improvement can be attributed to the early engagement of epipolar constraints, which effectively eliminates geometry inconsistencies among matches. The incorporation of geometry verification during prediction results in more accurate and robust matches, as visually demonstrated in Figure~\ref{Visualization}.

% \section{Augmentation For Cross View Images}

\section{Track Length Distribution}

Track length measures the number of consecutive frames in which a feature point in the scene can be reliably tracked, reflecting the quality of a reconstructed model. Longer track length implies more accurate reconstruction and more robust feature points. Table~\ref{tab:track} shows that our method achieves longer track length on average. The distribution of the track length for all methods is shown in Figure~\ref{fig:track_dist}, where the x-axis is the track length and the y-axis is the frequency. Our method demonstrates a more consistent track length distribution compared to other methods.

\begin{table}[!ht]
    \centering
    \resizebox{0.47\textwidth}{!}{%
    \begin{tabular}{cccccccc}
    \Xhline{1pt}
     & SIFT~\cite{Lowe:2004:DIF:993451.996342} & SP~\cite{superpoint2018}+SG~\cite{sarlin20superglue} & ALIKED~\cite{zhao2023aliked}+LG~\cite{lindenberger2023lightglue} & DKM~\cite{edstedt2023dkm} & RoMa~\cite{edstedt2024roma} & Ours \\
    \midrule
    Track Length & 12.74 & 13.06 & 21.3 & 3.04 & 3.12 & 23.74\\
    \bottomrule
    \end{tabular}
    }
    \caption{Average track length on IMC 2021~\cite{Jin2020}. Results are averaged across different scenes.}
    \label{runtime}
\label{tab:track}
\end{table}

\section{Failure Cases}
\paragraph{Distortion} When images are from different camera models, such as fisheye and perspective cameras, our pipeline would generate two separate models. One model primarily consists of perspective images with a few fisheye images, while the other predominantly contains fisheye images with a few perspective images.

\paragraph{Incorrect Initial Matches} Our pipeline relies on a backbone model for fundamental matrix estimation. If the initial matches provided by the backbone model are misleading, the pipeline may produce dense correspondences that are not necessarily correct, leading to inaccurate 3D reconstructions. A common failure case occurs with repetitive patterns, particularly symmetrical buildings.
